# Supplementary material for: Invariant Feature Regularization for Fair Face Recognition
Source: arXiv:2310.14652 source file (2023-10-23)
Supplement: Supplementary file 1 [file 8_appendix.tex]

\clearpage

\setcounter{section}{0}
\setcounter{figure}{0}
\setcounter{table}{0}

\noindent\textbf{\Large Appendix}
\vspace{0.1in}

This appendix is organized as follows:

\begin{itemize}
    \item Section~\ref{sec:a1} provides the method implementation details for partition learning with continuous partition matrix (Section 4.1) and different forms of classification loss $\mathcal{L}_{cls}$ (Section 4.2).
    \item Section~\ref{sec:a2} presents the experiment details of training settings and the estimation of demographic attribute labels with pretrained models (Section 5.1).
    \item Section~\ref{sec:a3} shows additional analysis and results. Specifically, Section~\ref{sec:a31} presents experiments with different $\mathcal{L}_{cls}$ and demographic attributes. Section~\ref{sec:a32} discusses ablation study on the choice of $\mathcal{L}_{inv}$ and settings of partition set $\mathcal{P}$ during feature learning, the effect of loss weight $\lambda$ during partition learning, as well as study of randomness sensitivity and model convergence (Section 5.4). Section~\ref{sec:a33} conveys analysis on causal effect learning and provides additional visualization results of partition subsets and failure cases (Section 5.5).
\end{itemize}

%------------------------------------------------------------
\section{Method Implementation in Section 4}
\label{sec:a1}
This section begins by presenting the implementation details of continuous partition matrix optimization in partition learning (Section 4.1), and then discusses various forms of classification loss $\mathcal{L}_{cls}$ in feature learning (Section 4.2).

%-----------------
\subsection{Partition Learning in Section 4.1}
\label{sec:a11-partition}
% 如何用soft partition matrix算supcon loss (Section 4.1)
During partition learning, we maximize the objective $\mathcal{L}_{inv}$ to obtain the partition matrix $\textbf{P}$ and the confounding demographic attribute. 
In practice, to enable back-propagation in optimization, we adopt a continuous partition matrix, \ie, soft partition denoted as $\tilde{\textbf{P}}\in\mathbb{R}^{C\times K}$.
Specifically, $\tilde{\textbf{P}}$ is initialized with random values and then updated using Eq. (4) in Section 4.1. 
After that, we threshold the learned soft partition matrix $\tilde{\textbf{P}}$ to obtain the hard partition matrix $\mathbf{P}\in \{0,1\}^{C\times K}$. 
\setlength{\abovedisplayskip}{3pt}\setlength{\belowdisplayskip}{3pt}
Denote the conventional Softmax function as $\mathcal{N}$, we apply Softmax normalization on $\tilde{\textbf{P}}$ such that:
\begin{equation}
    \mathcal{N} \left( \tilde{\textbf{P}}\right)_{i,k}  \in \left [ 0,1\right ],
    \text{\space and\space }
    \sum_{k=1}^K \mathcal{N} \left( \tilde{\textbf{P}}\right)_{i,k} =1, \forall i\in \{1...C\}.
    \label{eq:softmax}
\end{equation}
Here $\mathcal{N} \left( \tilde{\textbf{P}}\right)_{i,k}$ represents the confidence value of the $i$-th identity belonging to the $k$-th subset. 
Therefore, based on the confidence values of each subset, we re-weigh the computation of supervised contrastive loss~\cite{khosla2020supervised} $\mathcal{L}_{cls}$ in $\mathcal{L}_{inv}$ of Eq. (4), as formulated below:
\begin{equation}
    \begin{aligned}
        &\mathcal{L}_{cls}(\Phi, \cdot, \tilde{\textbf{P}}, k)=\\
        &\sum_{\mathbf{x} \in \mathcal{X}} 
        \mathcal{N}(\tilde{\textbf{P}})_{y,k}\cdot\sum_{\mathbf{x}^\textrm{+}\in \mathcal{X}} -\mathrm{log} \frac{e^{\Phi(\mathbf{x})^\intercal \Phi(\mathbf{x}^\textrm{+})}}
        {\mathop{\sum}_{\mathbf{x}^\textrm{*}\in \mathcal{X}}^{\mathbf{x}^\textrm{*}\neq{\mathbf{x}}} e^{\Phi(\mathbf{x})^\intercal \Phi(\mathbf{x}^\textrm{*})}},
    \end{aligned}
    \label{eq:soft_partition}
\end{equation}
where $\mathcal{X}=\{\mathbf{x}_i\}_{i=1}^N$ is the set of all the $N$ training images, $\mathbf{x}^+$ is the corresponding positive image sharing the same identity with $\mathbf{x}$ in $\mathcal{X}$. Thus we can enable back-propagation to optimize the partition matrix.
After learning soft partition $\tilde{\textbf{P}}$, the hard partition matrix $\textbf{P}$ can be obtained as below:
\begin{equation}
    \begin{aligned}
        \textbf{P}_{i,k}=\left\{\begin{array}{l} 0, \text{\space if \space} \mathcal{N} \left( \tilde{\textbf{P}}\right)_{i,k}  \leqslant 0.5; \\ 
        1, \text{\space otherwise}.
        \end{array}\right.
    \end{aligned}
    \label{eq:hard_partition}
\end{equation}

% MLP ???

%--------------
\subsection{Classification Loss $\mathcal{L}_{cls}$ in Section 4.2}
\label{sec:a12-loss}

For invariant feature learning, we optimize the objective $\mathcal{L}_{inv}$ in Eq. (6) where the definition of classification loss $\mathcal{L}_{cls}$ has a variety of options. As our \textsc{Inv-REg} is orthogonal to the existing face technologies, it can be plugged into the latest classification losses without further modification.
In this section, we first illustrate the mathematical forms of $\mathcal{L}_{cls}$ for Arcface and CIFP baselines adopted in Section 4. 
Furthermore, we provide additional examples of other marginal losses, including Cosface and Cosface-based CIFP variation. Experimental results using these two losses are presented in Section~\ref{sec:a31}.

\noindent\textbf{Arcface}. In margin-based losses, the objective is to optimize the decision boundary in angular space based on the L2 normalized weights and features. Denote the angle between the extracted feature $\Phi(\mathbf{x})$ and a certain weight vector of class $y$ as $\theta$, the corresponding angle is computed as $\theta_{y}=\mathrm{arccos}(\Phi(\mathbf{x}), f_{y})$.
The $\mathcal{L}_{cls}$ of Arcface loss~\cite{deng2019Arcface} is then formulated as:
\begin{equation}
    \begin{aligned}
        &\mathcal{L}_{cls}(\Phi, f, \mathbf{P}, k) =\\
        &-\sum_{\mathbf{x} \in \mathcal{X}_k} \mathrm{log} \frac{e^{s\cdot cos(\theta_{y_i}+m)}}
        {e^{s\cdot cos(\theta_{y_i}+m)}+\sum_{j=1, j\neq y_i}^{C}e^{s\cdot cos\theta_{j}}},
    \end{aligned}
\end{equation}
where $s$ is the scale factor, and $m$ is the addictive margin in angular space. 
The decision boundary between the current class $y_i$ and its negative classes ${j} (j\neq y_i)$ is decided by the margin $m$, where $m=0$ degenerates to the conventional Softmax cross-entropy loss, and $m>0$ guarantees the intra-class compactness and inter-class discriminability with minimum $m$ margin in feature space.
In practice $m$ is a predefined fixed value.

\noindent\textbf{CIFP}. Unlike Arcface which applies a fixed margin to all the samples, CIFP~\cite{xu2021consistent} assigns an adaptive margin to each instance based on the false positive rate (FPR) indicator, where hard samples (\ie, misclassified in training) have larger margin values. 
CIFP can be regarded as margin-based sample re-weighting to promote recognition consistency across different groups.
Depending on the utilized marginal losses, CIFP can have different variations. 
In Section 4, we adopted CIFP based on Arcface margin, and the corresponding $\mathcal{L}_{cls}$ is expressed as follows:
\begin{equation}
    \begin{aligned}
        &\mathcal{L}_{cls}(\Phi, f, \mathbf{P}, k) = \\
        &-\sum_{\mathbf{x} \in \mathcal{X}_k} \mathrm{log} \frac{e^{s\cdot cos(\theta_{y_i}+m)}}
        {e^{s\cdot cos(\theta_{y_i}+m)}+\sum_{j=1, j\neq y_i}^{C}e^{s\cdot cos\left(\theta_j+\frac{\gamma_i^+}{\gamma_u^+}\right)}},
    \end{aligned}
\end{equation}
where $\gamma_i^+$ and $\gamma_u^+$ are the instance FPR and overall FPR indicators respectively. Please refer to ~\cite{xu2021consistent} for more details.

\noindent\textbf{Cosface}. Both Arcface and Cosface~\cite{wang2018cosface} target maximizing inter-class variance and minimizing intra-class variance. However, Cosface removes the addictive margin to the outside of $cos(\theta)$ and applies it on the logit level as derived below. 
\begin{equation}
    \begin{aligned}
        &\mathcal{L}_{cls}(\Phi, f, \mathbf{P}, k) =\\
        &-\sum_{\mathbf{x} \in \mathcal{X}_k} \mathrm{log} \frac{e^{s\cdot (cos\theta_{y_i}+m)}}
        {e^{s\cdot (cos\theta_{y_i}+m)}+\sum_{j=1, j\neq y_i}^{C}e^{s\cdot cos\theta_{j}}}.
    \end{aligned}
\end{equation}

\noindent\textbf{CIFP-Cosface}. For the Cosface variation of CIFP, denoted as CIFP-Cosface, both the fixed margin and the adaptive FPR-based margin are applied on the logit level. The formula is given below. 
\begin{equation}
    \begin{aligned}
        &\mathcal{L}_{cls}(\Phi, f, \mathbf{P}, k) = \\
        &-\sum_{\mathbf{x} \in \mathcal{X}_k} \mathrm{log} \frac{e^{s\cdot (cos\theta_{y_i}+m)}}
        {e^{s\cdot (cos\theta_{y_i}+m)}+\sum_{j=1, j\neq y_i}^{C}e^{s\cdot \left(cos\theta_{j}+\frac{\gamma_i^+}{\gamma_u^+}\right)}}.
    \end{aligned}
\end{equation}

%------------------------------------------------------------
\section{Experiment Details}
\label{sec:a2}

This section discusses the details of training settings and the estimation of demographic attribute labels (Section 5.1). 

% ---------------------
\subsection{Training Settings}
\label{sec:a21}
% details of training settings, lr schedulers, margins, SGD settings, etc. (Section 5.1)
In the experiments, we employed SGD optimizer with momentum 0.9 and weight decay of 5e-4 to train the models. 
The learning rate started at 0.1 and was reduced by a factor of 10 after 110K, 190K, and 220K iterations.
The total number of training epochs was 21 for all the experiments.
We adopted the modified ResNet architecture ~\cite{he2016deep, deng2019arcface} as the backbone, 
where Batch Normalisation (BN), Dropout, fully connected layer, and BN were appended to the last convolutional layer as the output. The embedding size was 512.
For partition learning using Eq.~\ref{eq:soft_partition}, we referred to~\cite{khosla2020supervised} and appended a multi-layer perceptron to the backbone, which consists of a single hidden layer of size 512 and output vector of size 128.
For the training losses in feature learning, we configured the scale as 64 and the margin as 0.4 for Arcface and CIFP, and 0.35 for Cosface and CIFP-Cosface.
We adhered to the original work for the other settings in CIFP. 

% ---------------------
\subsection{Demographic Attributes Estimation}
\label{sec:a22}
\input{appendix/data}
% pretrained attribute classfication models, data cleaning [pts].
To analyze the demographic statistics of the training data in Section 5.1, as well as investigate the effect of ground-truth partitions in Section 5.4, we employed pretrained attribute classification models to estimate the demographic attributes.
In particular, the annotations of race (\ie, Caucasian, African, South Asian, and East Asian) and gender (\ie, female and male) for the MS-Celeb-1M dataset~\cite{deng2019Arcface,guo2016ms} were predicted. 
A majority voting strategy was employed in post-cleaning to ensure that images of the same identity have consistent demographic attributes.
Statistics of the cleaned attributes are shown in Table~\ref{tab:data}.
It is obvious that the dataset is heavily skewed towards Caucasian race and male gender with more samples and identities than the counterparts. 
This highly imbalanced distribution leads to a degradation of recognition fairness in conventional training.

%------------------------------------------------------------
\section{Additional Analysis and Results}
\label{sec:a3}

This section first presents experiments involving different $\mathcal{L}_{cls}$ and demographic attributes. It then discusses the ablation study on the choice of $\mathcal{L}_{inv}$, the setting of partition set $\mathcal{P}$, the loss weight $\lambda$ during partition learning, randomness sensitivity and model convergence. Finally, analysis on causal effect learning and additional visualization results are provided.

%------------------- experiments ------------------
\subsection{Additional Experiments}
\label{sec:a31}

\input{appendix/cosface}
\input{appendix/mfr}

\noindent\textbf{Results on Different $\mathcal{L}_{cls}$}. 
% Implement with Cosface
Referring to the definitions in ~\ref{sec:a12-loss}, we plugged our \textsc{Inv-Reg} into Cosface and CIFP-Cosface baselines. The models were trained with ResNet-50 backbone, and evaluated on MFR dataset. 
We observe in Table~\ref{tab:cosface} that, our method demonstrates superiority over both baselines with improved average accuracy and reduced standard deviation. Moreover, the performance of underrepresented minority racial groups is greatly enhanced without sacrificing the majority accuracy. This validates that our method is orthogonal to diverse loss functions and brings further performance benefits.

\noindent\textbf{Results on Children and Masked Faces}.
% MFR results on more attributes (R50:  children, masked faces)
In addition to multi-race attributes, we conducted evaluation on MFR dataset for children and masked face attributes. Children category contains 14K identities and 157K images, while masked faces category contains 6.9K identities with 6.9K masked images and 13K non-masked images. For the evaluation metric, true accept rate (TAR) with false accept rate (FAR) 1e-4 is obtained as in Table~\ref{tab:more attribtues}. 
Our \textsc{Inv-Reg} method outperforms the baselines on both attributes regardless of the marginal losses, demonstrating its generalization ability under diverse demographic attributes.

%\noindent\textbf{Results on race-balanced data}
% BUPT results

% IJBC evaluation with attributes?

%------------------- ablation ------------------
\subsection{Additional Ablation Study}
\label{sec:a32}

\input{appendix/Linv_loss}

\noindent\textbf{Choice of $\mathcal{L}_{inv}$ in Eq. (6)}.
% We leave the ablation on $\mathcal{L}_{inv}$ in Appendix due to space constraint.
Section 3.2 discussed different implementations of $\mathcal{L}_{inv}$, including IRMv1~\cite{arjovsky2019invariant} in Eq. (2) and REx~\cite{krueger2021out} in Eq. (3).
To investigate the choice of $\mathcal{L}_{inv}$, we performed feature learning with both implementations. 
Table~\ref{tab:Linv} lists the evaluation results on MFR dataset with CIFP baseline and ResNet-50 backbone. 
We observe that, both implementations of $\mathcal{L}_{inv}$ greatly improve the multi-race performance with higher average accuracy and lower standard deviation compared with CIFP. This validates the effectiveness of invariant learning with IRM theory~\cite{arjovsky2019invariant}.
In addition, $\mathcal{L}_{inv}$ with IRMv1 achieves the top performance on most attributes, especially on minority races (\eg, improving East Asian from 55.74 to 57.82). Thus we adopted IRMv1 in our experiments.

\input{appendix/figure_lambda_partition}
\input{appendix/figure_lambda_curve}

\noindent\textbf{Loss Weight $\lambda$ in Eq. (4)}.
% ablation study of hyper-params \lambda in maximization stage
Section 5.4 presented the ablation of loss weight $\lambda$ in $\mathcal{L}_{inv}$ for feature learning. 
Here we further study the effect of $\lambda$ for partition learning.
We increased $\lambda$ from 0.1 to 0.7 and analyzed the resulted partition subsets and verification accuracy on MFR.
Figure~\ref{fig:lambda_partition} shows that the distribution of demographic attributes among partition subsets remains relatively consistent across various $\lambda$.
For example, subset 1) is dominated by African people and Caucasian and South Asian females in all the settings. 
Furthermore, Figure~\ref{fig:lambda_curve} depicts the average multi-race accuracy using different $\lambda$, where our method demonstrates robustness by maintaining stable accuracy levels.
The best performing $\lambda=0.2$ is adopted.

\input{appendix/single_partition}
\noindent\textbf{Partition set $\mathcal{P}$}.
% not maintain the previous P 
Table~\ref{tab:single_partition} lists the performance comparison using different settings in the partition set $\mathcal{P}$, \ie, retaining all previously discovered partitions as described in Section 5, or keeping only the most recent partition.
We observe that both settings result in performance improvement over the Arcface baseline with ResNet-50 backbone, yet maintaining all previously discovered partitions yields superior accuracy.
 We postulate that model trained solely on the most recent partition may again exhibit bias towards previously deconfounded demographic attributes in earlier partitions. This is due to the model's tendency to overfit to the confounding demographic-specific features. On the other hand, by maintaining all the learned partitions in $\mathcal{P}$, diverse demographic biases will be mitigated progressively in the trained models, improving the robustness across all demographic groups. 
 
\input{appendix/std}
\noindent\textbf{Sensitivity to randomness}.
% sensitivity of std to random seeds
 In the experiments, we utilized Std to evaluate model fairness on different demographic groups. To address the variability of the Std metric due to randomness, we performed sensitivity study on MFR dataset with 5 random seeds in Table~\ref{tab:std}, and the low variability validates the significance of our results.

\input{appendix/epoch}
\noindent\textbf{Model Convergence}.
% more partition with longer training epoch
In Table~\ref{tab:convergence}, we extended Table 9 results by training CIFP and our method with more epochs. CIFP hardly benefits from more training, validating that it converges at 21 epoch. In contrast, our method with more partitions brings further improvement given more epochs, validating that more partitions requires larger number of training epochs to fully converge.

%------------------- Analysis ------------------
\subsection{Additional Analysis}
\label{sec:a33}
\input{appendix/figure_par2}
\input{appendix/figure_par3}
\input{appendix/figure_par4}
\noindent\textbf{Learning Causal Effect}. The causal effect from the image $X$ to prediction $Y$ is given by $P(Y|do(X))$~\cite{pearl2009causality}. In Figure 3, $P(Y|do(X))$ can be expanded using the backdoor adjustment formula:
\setlength{\abovedisplayskip}{3pt}\setlength{\belowdisplayskip}{3pt}
\begin{equation}
    P(Y|do(X)) = \sum_d P(Y|X,d)P(D=d),
\end{equation}
which corresponds to learning $P(Y|X,d)$ within each confounder stratum (\ie, demographic group), and combining them with the fixed population-level prior $P(D)$. In contrast, conventional learning using the full training data corresponds to maximizing the likelihood $P(Y|X)$, given by:
\begin{equation}
    P(Y|X) = \sum_d P(Y|X,d)P(D=d|X),
\end{equation}

where the key difference is that the weight of each $P(Y|X,d)$ changes from the population-specific $P(D=d)$ to the sample-specific $P(D=d|X)$. However, the appearance of $X$ is affected by $D$, $P(D=d|X)$ tends to have an extremely large value on the demographic group $D=d$ that $X$ belongs to.

Hence when group $d$ contains spurious demographic-specific context, the training can be dominated by $P(Y|X,d)$, such that the model recklessly captures the context for prediction.
Note that the key to capture the causal effect $P(Y|do(X))$ is \emph{not} to learn a representation independent from the demographic attributes,
but to fairly adjust the contribution of each $P(Y|X,d)$ by $P(D=d)$, where $d$ indeed participates in the prediction by $P(Y|X,d)$, \ie, the demographic attribute contains valid cue to differentiate identities.

\noindent\textbf{Visualization of Partition Subsets}.
% visualize the face images in partition subsets
In Figure 7, we presented the demographic distribution of different partition subsets. Here we further visualized the face images in each subset as shown in Figure~\ref{fig:partition2}. 
There exhibits a distinct contrast between the two subsets in each partition. For instance, in the first partition, subset 1) is primarily composed of male faces whereas subset 2) contains mostly female images. This further verifies our analysis in Section 5.5 that each partition encodes a certain demographic attribute. 
In addition, we extended our analysis to visualize the partition results when more than two subsets are utilized (Table 8), \ie, number of subsets $K=3$ and $K=4$ as shown in Figure~\ref{fig:partition3} and Figure~\ref{fig:partition4}, respectively.
We can see that subsets of $K=3$ behave with different preferences in the demographic attributes, where subset 1) and 2) are dominated by Caucasian males and females respectively, while all other attributes are categorized into subset 3).
As for $K=4$, in addition to the attributes of race and gender, age is also considered during partition learning. As an illustration, both subset 2) and 3) consist mostly males of Caucasian and South Asian, yet the faces in subset 2) are older in age compared to those in subset 3). 

\input{appendix/figure_facepair}

\noindent\textbf{Failure Cases Analysis}. We supplement more visualization results on failure cases using RFW dataset. 
Due to factors such as hairstyle, wearing hat, and head poses, Arcface baseline presents low similarity scores for faces from the same identity as shown in Figure~\ref{fig:6a}, yet high similarity values for the negative face pairs of different identities in Figure~\ref{fig:6b}.
In comparison, our \textsc{Inv-Reg} effectively captures the causal feature that is invariant of the spurious demographic-specific attributes, resulting in improved positive similarity and decreased negative similarity scores.

%------------------------------------------------------------
